# Supplementary material for: Structured Prompt Tuning
Source: arXiv:2205.12309 source file (2022-05-24)
Supplement: Supplementary file 1 [file appendix.tex]

\section{Additional Training Details}
\label{additional}
